# Supplementary material for: Resonant Raman scattering theory for Kitaev models and their Majorana fermion boundary modes
Source: arXiv:1606.02189 ancillary file (2016-06-07)
Supplement: Supplementary file 1 [file Kitaev_Couplings_Derivation_minimal3.pdf]

# Resonant Raman Terms For Kitaev Iridates

This notebook was written by Brent Perreault and is intended to go along with his papers that uses Resonant Raman in the Kitaev Model. Here we focus on the (near) ideal iridate structure to see at which orders the chiral three-spin terms that project into the zero flux sector appear.

Running the whole notebook takes my laptop ~20 mins, primarily due to the Simplify commands that are used before outputting results, and specifically the ones in the last section. There are time markers at every section and at a couple of slow spots indicating the number of seconds since the start (There are 4 sections, the first three sections run in 44 seconds, the last line takes ~15mins).

The operations of tensor multiplication are carefully optimized for efficient evaluation. In fact we use a homemade function for this

`TensorMultiply[A, B, {{a1, b1}, {a2, b2}, ...}]`

yields the tensor product of tensors A and B in the pairs {a<sub>i1</sub>, b<sub>i2</sub>} of slots.

*based off of an answer by m\_goldberg on question 77511 from azag0 on mathematica.stackexchange.com*

```
TensorMultiply[A_, B_, pairs_] := Activate@
  TensorContract[Inactive[TensorProduct][A, B], (# + {0, TensorRank[A]}) & /@ pairs];
```

---

## Initialization, Data, and Setup

```
start = SessionTime[];
```

Using the Clebsch-Gordon coefficients and separately adding spin and orbital angular momenta, and then requiring anti-symmetry of the resulting (and initial) states leads to the following matrix mapping between the LS states of {S (1) ; P (3x3) ; D (5)}, where the numbering goes from higher angular momentum to lower, changing lz before sz, to the basis of distinct ls product states given by

$\{(\frac{1}{2}, -\frac{1}{2}), (\frac{1}{2}, \frac{1}{2}), (-\frac{1}{2}, -\frac{1}{2})\}, \{(9, 3, 3)\}$  where the right spin's angular momentum is counted downward before the left one.

$$CG = \begin{pmatrix} 0 & 0 & 0 & 0 & 0 & 0 & 0 & 0 & 0 & 0 & 1 & 0 & 0 & 0 & 0 \\ 0 & 0 & 0 & 0 & \frac{1}{\sqrt{2}} & 0 & 0 & 0 & 0 & 0 & 0 & \frac{1}{\sqrt{2}} & 0 & 0 & 0 \\ \frac{1}{\sqrt{3}} & 0 & 0 & 0 & 0 & \frac{1}{\sqrt{2}} & 0 & 0 & 0 & 0 & 0 & 0 & \frac{1}{\sqrt{6}} & 0 & 0 \\ 0 & 0 & 0 & 0 & -\frac{1}{\sqrt{2}} & 0 & 0 & 0 & 0 & 0 & \frac{1}{\sqrt{2}} & 0 & 0 & 0 & 0 \\ -\frac{1}{\sqrt{3}} & 0 & 0 & 0 & 0 & 0 & 0 & 0 & 0 & 0 & 0 & \sqrt{\frac{2}{3}} & 0 & 0 & 0 \\ 0 & 0 & 0 & 0 & 0 & 0 & \frac{1}{\sqrt{2}} & 0 & 0 & 0 & 0 & 0 & \frac{1}{\sqrt{2}} & 0 & 0 \\ \frac{1}{\sqrt{3}} & 0 & 0 & 0 & 0 & -\frac{1}{\sqrt{2}} & 0 & 0 & 0 & 0 & 0 & 0 & \frac{1}{\sqrt{6}} & 0 & 0 \\ 0 & 0 & 0 & 0 & 0 & 0 & -\frac{1}{\sqrt{2}} & 0 & 0 & 0 & 0 & 0 & 0 & \frac{1}{\sqrt{2}} & 0 \\ 0 & 0 & 0 & 0 & 0 & 0 & 0 & 0 & 0 & 0 & 0 & 0 & 0 & 0 & 1 \\ 0 & 1 & 0 & 0 & 0 & 0 & 0 & 0 & 0 & 0 & 0 & 0 & 0 & 0 & 0 \\ 0 & 0 & 1 & 0 & 0 & 0 & 0 & 0 & 0 & 0 & 0 & 0 & 0 & 0 & 0 \\ 0 & 0 & 0 & -1 & 0 & 0 & 0 & 0 & 0 & 0 & 0 & 0 & 0 & 0 & 0 \\ 0 & 0 & 0 & 0 & 0 & 0 & 0 & -1 & 0 & 0 & 0 & 0 & 0 & 0 & 0 \\ 0 & 0 & 0 & 0 & 0 & 0 & 0 & 0 & 1 & 0 & 0 & 0 & 0 & 0 & 0 \\ 0 & 0 & 0 & 0 & 0 & 0 & 0 & 0 & 0 & 1 & 0 & 0 & 0 & 0 & 0 \end{pmatrix};$$

`CG.Transpose[CG] == IdentityMatrix[15]`

True

From the J basis to the Im basis (diagonalizes the 1-particle Kanamori Hamiltonian)

$$JJ2 = \text{ConjugateTranspose} \left[ \begin{pmatrix} 0 & 0 & 1 & 0 & 0 & 0 \\ -i\sqrt{\frac{1}{3}} & 0 & 0 & -i\sqrt{\frac{2}{3}} & 0 & 0 \\ 0 & \sqrt{\frac{2}{3}} & 0 & 0 & \sqrt{\frac{1}{3}} & 0 \\ \sqrt{\frac{2}{3}} & 0 & 0 & -\sqrt{\frac{1}{3}} & 0 & 0 \\ 0 & i\sqrt{\frac{1}{3}} & 0 & 0 & -i\sqrt{\frac{2}{3}} & 0 \\ 0 & 0 & 0 & 0 & 0 & 1 \end{pmatrix} \right];$$

`JJ2.ConjugateTranspose[JJ2] == IdentityMatrix[6]`

True

from the XYZ basis to Im [with {up,down} blocks]

$$L = \text{Conjugate} \left[ \begin{pmatrix} \frac{1}{\sqrt{2}} & \frac{i}{\sqrt{2}} & 0 & 0 & 0 & 0 \\ 0 & 0 & i & 0 & 0 & 0 \\ \frac{1}{\sqrt{2}} & -\frac{i}{\sqrt{2}} & 0 & 0 & 0 & 0 \\ 0 & 0 & 0 & \frac{1}{\sqrt{2}} & \frac{i}{\sqrt{2}} & 0 \\ 0 & 0 & 0 & 0 & 0 & i \\ 0 & 0 & 0 & \frac{1}{\sqrt{2}} & -\frac{i}{\sqrt{2}} & 0 \end{pmatrix} \right];$$

**\$Assumptions = t1 ∈ Reals && t2 ∈ Reals && t3 ∈ Reals && t4 ∈ Reals && ta ∈ Reals && ts ∈ Reals**

t1 ∈ Reals && t2 ∈ Reals && t3 ∈ Reals && t4 ∈ Reals && ta ∈ Reals && ts ∈ Reals

Hopping matrix T in the X = zy, Y = xz, Z = xy basis.

$$T_z = \begin{pmatrix} t_1 & t_2 & t_4 & 0 & 0 & 0 \\ t_2 & t_1 & t_4 & 0 & 0 & 0 \\ t_4 & t_4 & t_3 & 0 & 0 & 0 \\ 0 & 0 & 0 & t_1 & t_2 & t_4 \\ 0 & 0 & 0 & t_2 & t_1 & t_4 \\ 0 & 0 & 0 & t_4 & t_4 & t_3 \end{pmatrix};$$

$$T_y = \begin{pmatrix} t_1 & t_4 & t_2 & 0 & 0 & 0 \\ t_4 & t_3 & t_4 & 0 & 0 & 0 \\ t_2 & t_4 & t_1 & 0 & 0 & 0 \\ 0 & 0 & 0 & t_1 & t_4 & t_2 \\ 0 & 0 & 0 & t_4 & t_3 & t_4 \\ 0 & 0 & 0 & t_2 & t_4 & t_1 \end{pmatrix};$$

$$T_x = \begin{pmatrix} t_3 & t_4 & t_4 & 0 & 0 & 0 \\ t_4 & t_1 & t_2 & 0 & 0 & 0 \\ t_4 & t_2 & t_1 & 0 & 0 & 0 \\ 0 & 0 & 0 & t_3 & t_4 & t_4 \\ 0 & 0 & 0 & t_4 & t_1 & t_2 \\ 0 & 0 & 0 & t_4 & t_2 & t_1 \end{pmatrix};$$

**TLz = L.Tz.ConjugateTranspose[L] // FullSimplify;**

**TJz = JJ2.TLz.Inverse[JJ2];**

**TLx = L.Tx.ConjugateTranspose[L] // FullSimplify;**

**TJx = JJ2.TLx.Inverse[JJ2];**

**TLy = L.Ty.ConjugateTranspose[L] // FullSimplify; TJy = JJ2.TLy.Inverse[JJ2];**

Note that there is not hopping from low energy subspace to low energy subspace with just t2 ( $J_{\text{eff}} = 1/2$  is the first two rows/columns)

**TJz /. {t1 → 0, t3 → 0, t4 → 0} // MatrixForm**

$$\begin{pmatrix} 0 & 0 & 0 & 0 & 0 & -i\sqrt{\frac{2}{3}}t_2 \\ 0 & 0 & i\sqrt{\frac{2}{3}}t_2 & 0 & 0 & 0 \\ 0 & -i\sqrt{\frac{2}{3}}t_2 & 0 & 0 & -\frac{it_2}{\sqrt{3}} & 0 \\ 0 & 0 & 0 & 0 & 0 & \frac{it_2}{\sqrt{3}} \\ 0 & 0 & \frac{it_2}{\sqrt{3}} & 0 & 0 & 0 \\ i\sqrt{\frac{2}{3}}t_2 & 0 & 0 & -\frac{it_2}{\sqrt{3}} & 0 & 0 \end{pmatrix}$$

This maps the indices for 1-particle products states into indices for 2-particle (anti-symmetrized) states

```

m = Table[0, {s, 6}, {t, 6}];
m[[1, 4]] = 1; m[[4, 1]] = 1;
m[[1, 5]] = 2; m[[5, 1]] = 2;
m[[1, 6]] = 3; m[[6, 1]] = 3;
m[[2, 4]] = 4; m[[4, 2]] = 4;
m[[2, 5]] = 5; m[[5, 2]] = 5;
m[[2, 6]] = 6; m[[6, 2]] = 6;
m[[3, 4]] = 7; m[[4, 3]] = 7;
m[[3, 5]] = 8; m[[5, 3]] = 8;
m[[3, 6]] = 9; m[[6, 3]] = 9;
m[[1, 2]] = 10; m[[2, 1]] = 10;
m[[1, 3]] = 11; m[[3, 1]] = 11;
m[[2, 3]] = 12; m[[3, 2]] = 12;
m[[4, 5]] = 13; m[[5, 4]] = 13;
m[[4, 6]] = 14; m[[6, 4]] = 14;
m[[5, 6]] = 15; m[[6, 5]] = 15;
m // MatrixForm

```

$$\begin{pmatrix} 0 & 10 & 11 & 1 & 2 & 3 \\ 10 & 0 & 12 & 4 & 5 & 6 \\ 11 & 12 & 0 & 7 & 8 & 9 \\ 1 & 4 & 7 & 0 & 13 & 14 \\ 2 & 5 & 8 & 13 & 0 & 15 \\ 3 & 6 & 9 & 14 & 15 & 0 \end{pmatrix}$$

Pauli Matrices

```

sigma = Table[0, {n, 1, 3}, {a, 1, 2}, {b, 1, 2}];
sigma[[1]] =  $\begin{pmatrix} 0 & 1 \\ 1 & 0 \end{pmatrix}$ ; sigma[[2]] =  $\begin{pmatrix} 0 & -i \\ i & 0 \end{pmatrix}$ ; sigma[[3]] =  $\begin{pmatrix} 1 & 0 \\ 0 & -1 \end{pmatrix}$ ;
TensorDimensions[sigma]
MatrixForm /@ sigma

```

$$\{3, 2, 2\}$$

$$\left\{ \begin{pmatrix} 0 & 1 \\ 1 & 0 \end{pmatrix}, \begin{pmatrix} 0 & -i \\ i & 0 \end{pmatrix}, \begin{pmatrix} 1 & 0 \\ 0 & -1 \end{pmatrix} \right\}$$

Low-energy Pauli tensors in 6x6 form and a 3x3 LeviCivita to convert two same-site spins to one

```

sigma6 =  $\begin{pmatrix} 1 & 0 \\ 0 & 1 \\ 0 & 0 \\ 0 & 0 \\ 0 & 0 \\ 0 & 0 \end{pmatrix}$ .TensorTranspose[sigma, {2, 1, 3}]. $\begin{pmatrix} 1 & 0 & 0 & 0 & 0 & 0 \\ 0 & 1 & 0 & 0 & 0 & 0 \end{pmatrix}$ ;
ee = LeviCivitaTensor[3];

```

The eigenergies of the 2-particle states, and the diagonal Hamiltonian matrix

```
Clear[J]
Et = (U - 3 J); Es = (U - J); Ed = (U + 2 J);
HintM = DiagonalMatrix[{Ed, Et, Et, Et, Et, Et, Et, Et, Et, Et, Es, Es, Es, Es, Es}];
```

The Effective Hamiltonian in the  $|s\rangle$ -basis

```
Heff = CG.Inverse[HintM].ConjugateTranspose[CG];
CGI = Transpose[Inverse[CG]];
```

The effective Hamiltonian is diagonal in the S and D parts but not in the P (triplet) parts

The 4-tensor in the 1-particle J basis for interaction of incoming a with b,bb and outgoing aa

```
M = Table[If[a != b && aa != bb, Heff[m[a, b], m[bb, aa]] Sign[a - b] Sign[bb - aa], 0],
  {a, 1, 6}, {b, 1, 6}, {bb, 1, 6}, {aa, 1, 6}];
```

Change bases so that the indices are in the J basis (it comes out with order a, aa, b, bb)

```
JJ2I = ConjugateTranspose[JJ2];
MJ = TensorMultiply[TensorProduct[Conjugate[JJ2I], JJ2I],
  ConjugateTranspose[JJ2I].M.JJ2I, {{1, 2}, {3, 3}}];
TensorDimensions[MJ]
{6, 6, 6, 6}
```

Tensor with  $\sigma_{b,bb}^\mu$  to convert the local fermion to a (low-energy) spin

```
MM = -TensorTranspose[Sum[TensorProduct[TensorTranspose[MJ, {3, 4, 1, 2}][[b, bb]],
  TensorTranspose[sigma, {3, 1, 2}][[bb, b]]], {b, 1, 2}, {bb, 1, 2}], {1, 3, 2}];
TensorDimensions[MM]
{6, 3, 6}
```

Another interaction tensor, MM2, for spin interaction on a single site with a holon hop elsewhere in the middle that keeps the excited electron on the same site for two hops

```

Heff2 = CG.(Inverse[HintM])2.ConjugateTranspose[CG];
M22 = Table[
  If[a ≠ b && aa ≠ bb, Heff2[[m[[a, b]], m[[bb, aa]]]] Sign[a - b] Sign[bb - aa], 0],
  {a, 1, 6}, {b, 1, 6}, {bb, 1, 6}, {aa, 1, 6}];
MJ2 = TensorMultiply[TensorProduct[Conjugate[JJ2I], JJ2I],
  ConjugateTranspose[JJ2I].M22.JJ2I, {{1, 2}, {3, 3}}];
MM2 = -TensorTranspose[Sum[TensorProduct[TensorTranspose[MJ2, {3, 4, 1, 2}][[b, bb]],
  TensorTranspose[sigma, {3, 1, 2}][[bb, b]]], {b, 1, 2}, {bb, 1, 2}], {1, 3, 2}];

SessionTime[] - start
0.7851046

```

## Exchange parameters for the 2-hop processes

(LF, or NN exchange)

We focus on a z-bond

```

Hz = 2 Sum[TensorProduct[TensorTranspose[sigma, {3, 1, 2}][[aa, a]],
  TensorTranspose[TJz.MM.TJz, {1, 3, 2}][[a, aa]]], {a, 1, 2}, {aa, 1, 2}];

```

```

Jterm = (Hz[[1, 1]] + Hz[[2, 2]]) / 2 // FullSimplify
(4 (J2 (4 t12 - 4 t1 t3 + 3 (t32 + 4 t42)) + 2 J (2 t12 + t32 + 3 t42) U - (2 t1 + t3)2 U2)) /
(9 (J - U) (3 J - U) (2 J + U))

```

```

Kterm = Hz[[3, 3]] - Jterm // FullSimplify
8 J ((t1 - t3)2 - 3 (t2 - t4) (t2 + t4))
- (9 (3 J2 - 4 J U + U2))

```

```

GammaTerm = Hz[[1, 2]] // FullSimplify
8 J (2 t1 t2 - 2 t2 t3 + 3 t42)
- (9 (3 J2 - 4 J U + U2))

```

```

GammaPterm = Hz[[1, 3]] // FullSimplify
8 J (t1 - 3 t2 - t3) t4
- (9 (3 J2 - 4 J U + U2))

```

```

Series[Jterm, {J, 0, 1}]
4 (4 t12 + 4 t1 t3 + t32) / 9 U - 8 (2 t12 + 4 t1 t3 - 3 t42) J / 9 U2 + O[J]2

```

These all check out with 1310.7940v3. Next I will check the symmetry related bonds just to make sure

```

Hx = 2 Sum[TensorProduct[TensorTranspose[sigma, {3, 1, 2}][[aa, a]],
  TensorTranspose[TJx.MM.TJx, {1, 3, 2}][[a, aa]]], {a, 1, 2}, {aa, 1, 2}];

```

$$\begin{pmatrix} 0 & 0 & 1 \\ 0 & 1 & 0 \\ 1 & 0 & 0 \end{pmatrix} \cdot H_x \cdot \begin{pmatrix} 0 & 0 & 1 \\ 0 & 1 & 0 \\ 1 & 0 & 0 \end{pmatrix} - H_z \text{ // FullSimplify}$$

{0, 0, 0}, {0, 0, 0}, {0, 0, 0}

y-bond just for completion

```
Hy = 2 Sum[TensorProduct[TensorTranspose[sigma, {3, 1, 2}][[aa, a]],
  TensorTranspose[TJy.MM.TJy, {1, 3, 2}][[a, aa]], {a, 1, 2}, {aa, 1, 2}];
```

$$\begin{pmatrix} 1 & 0 & 0 \\ 0 & 0 & 1 \\ 0 & 1 & 0 \end{pmatrix} \cdot H_y \cdot \begin{pmatrix} 1 & 0 & 0 \\ 0 & 0 & 1 \\ 0 & 1 & 0 \end{pmatrix} - H_z \text{ // FullSimplify}$$

{0, 0, 0}, {0, 0, 0}, {0, 0, 0}

These all check out, as shown by the vanishing of the previous difference matrices.

```
SessionTime[] - start
```

3.6976337

## 3-hop processes

Next are 3-bond loops with three hops. One of the hops is along a second neighbor bond. We compute the case of a z-type NNN bond here (the other ones follow by symmetry)

The hopping on a NNN y-bond

$$Tz2 = \begin{pmatrix} 0 & ts & 0 & 0 & 0 & 0 \\ ts + ta & 0 & 0 & 0 & 0 & 0 \\ 0 & 0 & 0 & 0 & 0 & 0 \\ 0 & 0 & 0 & 0 & ts & 0 \\ 0 & 0 & 0 & ts + ta & 0 & 0 \\ 0 & 0 & 0 & 0 & 0 & 0 \end{pmatrix};$$

```
TLz2 = L.Tz2.ConjugateTranspose[L] // FullSimplify; (* L basis *)
```

```
TJz2 = JJ2.TLz2.Inverse[JJ2]; (* J basis *)
```

```
(* from J basis to L basis *)
```

We first deal with processes with intermediate doublon hops

Consider first the  $(a_2)$  and  $(a_2')$  processes that have the doublon hopping on the z-bond, and the incoming on the y (x) bond respectively.

$$Hza_2 = T^x M T^{z2} M T^y \sigma \quad (312)$$

```
Mza2 = TJx.MM.TJz2.MM.TJy;
```

```
Hza2 =
```

```
TensorTranspose[Sum[TensorProduct[TensorTranspose[Mza2, {1, 3, 4, 2}][[aa, a]],
  TensorTranspose[sigma, {3, 1, 2}][[a, aa]], {a, 1, 2}, {aa, 1, 2}], {3, 1, 2}];
```

The terms that vanish at this order in J (given all NN hopping possibilities) are [in the order  $S_3 S_2 S_1$ , matrices are read row then column for indices from left to right]

xyz , xzy , zxy, zyx

$$Hza2' = T^y M (T^{z2})^T M T^x \sigma \quad (132)$$

```
Mza2p = TJy.MM.ConjugateTranspose[TJz2].MM.TJx;
```

```
Hza2p =
```

```
TensorTranspose[Sum[TensorProduct[TensorTranspose[Mza2p, {1, 3, 4, 2}][[aa, a]],
TensorTranspose[sigma, {3, 1, 2}][[a, aa]]], {a, 1, 2}, {aa, 1, 2}], {1, 3, 2}];
```

Now consider the  $(a_1)$  and  $(a_1')$  diagrams in which the doublon is on the x-bond

$$Hza1 = T^y M T^x M T^{z2} \sigma \quad (\text{order } 231)$$

```
Mza1 = TJy.MM.TJx.MM.TJz2;
```

```
Hza1 =
```

```
TensorTranspose[Sum[TensorProduct[TensorTranspose[Mza1, {1, 3, 4, 2}][[aa, a]],
TensorTranspose[sigma, {3, 1, 2}][[a, aa]]], {a, 1, 2}, {aa, 1, 2}], {2, 3, 1}];
```

$$Hza1' = (T^{z2})^T M T^x M T^y \sigma \quad (\text{order } 321)$$

```
Mza1p = ConjugateTranspose[TJz2].MM.TJx.MM.TJy;
```

```
Hza1p =
```

```
TensorTranspose[Sum[TensorProduct[TensorTranspose[Mza1p, {1, 3, 4, 2}][[aa, a]],
TensorTranspose[sigma, {3, 1, 2}][[a, aa]]], {a, 1, 2}, {aa, 1, 2}], {3, 2, 1}];
```

Now consider the  $(a_3)$  and  $(a_3')$  diagrams in which the doublon is on the y-bond

$$Hza3 = T^{z2} M T^y M T^x \sigma \quad (\text{order } 123)$$

```
Mza3 = TJz2.MM.TJy.MM.TJx;
```

```
Hza3 =
```

```
TensorTranspose[Sum[TensorProduct[TensorTranspose[Mza3, {1, 3, 4, 2}][[aa, a]],
TensorTranspose[sigma, {3, 1, 2}][[a, aa]]], {a, 1, 2}, {aa, 1, 2}], {1, 2, 3}];
```

$$Hza3' = T^x M T^y M (T^{z2})^T \sigma \quad (\text{order } 213)$$

```
Mza3p = TJx.MM.TJy.MM.ConjugateTranspose[TJz2]; Hza3p =
```

```
TensorTranspose[Sum[TensorProduct[TensorTranspose[Mza3p, {1, 3, 4, 2}][[aa, a]],
TensorTranspose[sigma, {3, 1, 2}][[a, aa]]], {a, 1, 2}, {aa, 1, 2}], {2, 1, 3}];
```

```
Hza1[[2, 3, 1]] // FullSimplify
```

$$\frac{1}{27 (2 J + U) (3 J^2 - 4 J U + U^2)^2} \left( 2 i J \left( J^2 \left( (-16 t_1 + 9 t_3 - 5 t_4) t_4 t_a - 6 t_4 (2 t_1 - 2 t_3 + t_4) t_s + 3 t_2^2 (t_a + 2 t_s) \right) - J \left( t_4 (12 t_1 - 7 t_3 + t_4) t_a - 3 t_2^2 t_s + 3 t_4 (2 t_1 - 2 t_3 + t_4) t_s \right) U + (3 t_2^2 + (8 t_1 - 5 t_3 - 3 t_4) t_4) t_a U^2 \right) \right)$$



**Hza1p[[2, 3, 1]] // FullSimplify**

$$-\frac{1}{27 (2 J + U) (3 J^2 - 4 J U + U^2)^2} \left( 2 i J \left( J^2 \left( (-16 t_1 + 9 t_3 - 5 t_4) t_4 t_a - 6 t_4 (2 t_1 - 2 t_3 + t_4) t_s + 3 t_2^2 (t_a + 2 t_s) \right) - J \left( t_4 (12 t_1 - 7 t_3 + t_4) t_a - 3 t_2^2 t_s + 3 t_4 (2 t_1 - 2 t_3 + t_4) t_s \right) U + (3 t_2^2 + (8 t_1 - 5 t_3 - 3 t_4) t_4) t_a U^2 \right) \right)$$

**Hza = (Hza2 - Hza2p + Hza1 - Hza1p + Hza3 - Hza3p);**

This is the term that projects into zero flux:

**Hza[[2, 3, 1]] // FullSimplify**

$$\frac{1}{27 (2 J + U) (3 J^2 - 4 J U + U^2)^2} \left( 4 i J \left( 2 J^2 (3 t_2^2 (4 t_a + 5 t_s) - t_4 (9 t_4 (t_a + t_s) - 2 t_3 (4 t_a + 5 t_s) + 2 t_1 (8 t_a + 5 t_s))) + J (3 t_2^2 (3 t_a + 5 t_s) - t_4 (26 t_1 t_a - 12 t_3 t_a + 6 t_4 t_a + 10 t_1 t_s - 10 t_3 t_s + 9 t_4 t_s)) U + 2 (3 t_2^2 + (10 t_1 - 4 t_3 - 3 t_4) t_4) t_a U^2 \right) \right)$$

This term multiplies the following coefficient in polarization space  $\epsilon_{in} \otimes \epsilon_{out}$ :  $(d_{23} \otimes d_{12} - d_{12} \otimes d_{23})$

Other terms appear at orders  $\frac{\omega}{\Delta}$

**MatrixForm[ @Simplify[SeriesCoefficient[Hza, {J, 0, 0}]]**

**MatrixForm[ @Simplify[J SeriesCoefficient[9 U^3 Hza, {J, 0, 1}]] // Factor**

$$\left\{ \begin{pmatrix} 0 & 0 & -\frac{4 i (2 t_1 + t_3)^2 t_a}{9 U^2} \\ 0 & 0 & 0 \\ \frac{4 i (2 t_1 + t_3)^2 t_a}{9 U^2} & 0 & 0 \end{pmatrix}, \begin{pmatrix} 0 & 0 & 0 \\ 0 & 0 & -\frac{4 i (2 t_1 + t_3)^2 t_a}{9 U^2} \\ 0 & \frac{4 i (2 t_1 + t_3)^2 t_a}{9 U^2} & 0 \end{pmatrix}, \right. \\ \left. \begin{pmatrix} -\frac{4 i (2 t_1 + t_3)^2 t_a}{9 U^2} & 0 & 0 \\ 0 & -\frac{4 i (2 t_1 + t_3)^2 t_a}{9 U^2} & 0 \\ 0 & 0 & -\frac{4 i (2 t_1 + t_3)^2 t_a}{9 U^2} \end{pmatrix} \right\} \\ \left\{ \begin{aligned} & -8 i J (t_2 (-t_4 t_a + t_3 t_s) - t_4 (t_4 t_a + t_3 t_s) + t_1 (-2 t_4 (t_a + t_s) + t_2 (t_a + 2 t_s) \\ & \frac{8}{3} i J (t_4 (-2 t_3 t_a + 3 t_4 t_a - 3 t_3 t_s) + t_2 (4 t_3 t_a + 3 t_4 t_a + 3 t_3 t_s) + t_1 (5 t_2 t_a + 2 t_4 t_a + 6 \\ & \frac{8}{3} i J (19 t_1^2 + 12 t_1 t_3 + 5 t_3^2 - 6 t_4^2) t_a \end{aligned} \right.$$

**SessionTime[] - start**

50.0260943

Now we consider the three hop processes involving a holon hop

Cosider first the  $(b_2)$  and  $(b_2')$  processes that have the holon hopping on the z-bond, and the incoming on the y (x) bond respectively.

$$H_{zb_2} = T^x \sigma T^{z2} M_2 T^y \sigma \quad (312)$$

```
Mzb2 = TJx.sigma6.TJz2.MM2.TJy;
```

```
Hzb2 =
```

```
TensorTranspose[Sum[TensorProduct[TensorTranspose[Mzb2, {1, 3, 4, 2}][[aa, a]],  
TensorTranspose[sigma, {3, 1, 2}][[a, aa]]], {a, 1, 2}, {aa, 1, 2}], {3, 1, 2}];
```

The terms that vanish at this order in J (given all NN hopping possibilities) are [in the order  $S_3 S_2 S_1$ , matrices are read row then column for indices from left to right]

xyz , xzy , zxy, zyx

$$H_{zb2}' = T^y \sigma (T^{z2})^T M2 T^x \sigma \quad (132)$$

```
Mzb2p = TJy.MM2.ConjugateTranspose[TJz2].sigma6.TJx;
```

```
Hzb2p =
```

```
TensorTranspose[Sum[TensorProduct[TensorTranspose[Mzb2p, {1, 3, 4, 2}][[aa, a]],  
TensorTranspose[sigma, {3, 1, 2}][[a, aa]]], {a, 1, 2}, {aa, 1, 2}], {1, 3, 2}];
```

Now consider the  $(c_1)$  and  $(c_1')$  diagrams in which the doublon is on the x-bond

$$H_{zb1} = T^y \sigma T^x M2 T^{z2} \sigma \quad (\text{order } 231)$$

```
Mzb1 = TJy.sigma6.TJx.MM2.TJz2;
```

```
Hzb1 =
```

```
TensorTranspose[Sum[TensorProduct[TensorTranspose[Mzb1, {1, 3, 4, 2}][[aa, a]],  
TensorTranspose[sigma, {3, 1, 2}][[a, aa]]], {a, 1, 2}, {aa, 1, 2}], {2, 3, 1}];
```

$$H_{zb1}' = (T^{z2})^T M2 T^x \sigma T^y \sigma \quad (\text{order } 321)$$

```
Mzb1p = ConjugateTranspose[TJz2].MM2.TJx.sigma6.TJy;
```

```
Hzb1p =
```

```
TensorTranspose[Sum[TensorProduct[TensorTranspose[Mzb1p, {1, 3, 4, 2}][[aa, a]],  
TensorTranspose[sigma, {3, 1, 2}][[a, aa]]], {a, 1, 2}, {aa, 1, 2}], {3, 2, 1}];
```

Now consider the  $(b_3)$  and  $(b_3')$  diagrams in which the doublon is on the y-bond

$$H_{zb3} = T^{z2} \sigma T^y M2 T^x \sigma \quad (\text{order } 123)$$

```
Mzb3 = TJz2.sigma6.TJy.MM2.TJx;
```

```
Hzb3 =
```

```
TensorTranspose[Sum[TensorProduct[TensorTranspose[Mzb3, {1, 3, 4, 2}][[aa, a]],  
TensorTranspose[sigma, {3, 1, 2}][[a, aa]]], {a, 1, 2}, {aa, 1, 2}], {1, 2, 3}];
```

$$H_{zb3}' = T^x M2 T^y \sigma (T^{z2})^T \sigma \quad (\text{order } 213)$$

```
Mzb3p = TJx.MM2.TJy.sigma6.ConjugateTranspose[TJz2]; Hzb3p =
```

```
TensorTranspose[Sum[TensorProduct[TensorTranspose[Mzb3p, {1, 3, 4, 2}][[aa, a]],  
TensorTranspose[sigma, {3, 1, 2}][[a, aa]]], {a, 1, 2}, {aa, 1, 2}], {2, 1, 3}];
```

$$H_{zb} = (H_{zb2} - H_{zb2p} + H_{zb1} - H_{zb1p} + H_{zb3} - H_{zb3p});$$

This is the term that projects into zero flux:

$$\text{Hzb}[[2, 3, 1]] // \text{FullSimplify}$$

$$\frac{8 i J (3 t^2 + (10 t_1 - 4 t_3 - 3 t_4) t_4) t_a (2 J - U)}{27 (3 J^2 - 4 J U + U^2)^2}$$

Each channel and its time-reversal pair are indeed equal up to a minus sign

$$\begin{aligned} & \text{Hza1} + \text{Hza1p} // \text{FullSimplify} \\ & \text{Hzb1} + \text{Hzb1p} // \text{FullSimplify} \\ & \{ \{ \{0, 0, 0\}, \{0, 0, 0\}, \{0, 0, 0\} \}, \\ & \quad \{ \{0, 0, 0\}, \{0, 0, 0\}, \{0, 0, 0\} \}, \{ \{0, 0, 0\}, \{0, 0, 0\}, \{0, 0, 0\} \} \} \\ & \{ \{ \{0, 0, 0\}, \{0, 0, 0\}, \{0, 0, 0\} \}, \\ & \quad \{ \{0, 0, 0\}, \{0, 0, 0\}, \{0, 0, 0\} \}, \{ \{0, 0, 0\}, \{0, 0, 0\}, \{0, 0, 0\} \} \} \\ & \text{Hz3} = \text{Hza} + \text{Hzb}; \\ & \text{MatrixForm} / @ \text{Simplify} [J \text{SeriesCoefficient} [9 U^3 \text{Hz3}, \{J, 0, 0\}]] // \text{Factor} \\ & \text{MatrixForm} / @ \text{Simplify} [J \text{SeriesCoefficient} [9 U^3 \text{Hz3}, \{J, 0, 1\}]] // \text{Factor} \\ & \text{MatrixForm} / @ \text{Simplify} [J^2 \text{SeriesCoefficient} [9 U^4 \text{Hz3}, \{J, 0, 2\}]] // \text{Factor} \\ & \left\{ \begin{pmatrix} 0 & 0 & 0 \\ 0 & 0 & 0 \\ 0 & 0 & 0 \end{pmatrix}, \begin{pmatrix} 0 & 0 & 0 \\ 0 & 0 & 0 \\ 0 & 0 & 0 \end{pmatrix}, \begin{pmatrix} 0 & 0 & 0 \\ 0 & 0 & 0 \\ 0 & 0 & 0 \end{pmatrix} \right\} \\ & \left\{ \begin{pmatrix} 0 & 0 & 0 \\ 0 & 0 & 0 \\ 0 & 0 & 0 \end{pmatrix}, \begin{pmatrix} 0 & 0 & 0 \\ 0 & 0 & 0 \\ 0 & 0 & 0 \end{pmatrix}, \begin{pmatrix} 0 & 0 & 0 \\ 0 & 0 & 0 \\ 0 & 0 & 0 \end{pmatrix} \right\} \\ & \left\{ \begin{aligned} & \frac{4}{3} i J^2 (-6 t_2 t_4 t_a - 6 t_4^2 t_a + t_2 t_3 t_s - 7 t_3 t_4 t_s + t_1 (8 t_2 t_a - 7 t_4 t_a + 1 \\ & - \frac{4}{3} i J^2 (t_4 (-4 t_3 t_a + 2 t_4 t_a - 3 t_3 t_s - 6 t_4 t_s) + t_2 (6 t_3 t_a + 8 t_4 t_a + 3 t_3 t_s + 6 t_4 t_s) + t_1 \\ & \frac{4}{3} i J^2 (t_4 (6 t_2 + 13 t_4) t_a + t_1^2 (-71 t_a + t_s) + t_3^2 (-19 t_a + t_s) - 2 t_1 t \end{aligned} \right. \end{aligned}$$

As in Ko et al, the doublon and holon hop channels cancel, but only at order  $J_H$ . Here, at order  $J_H^2$  we still have a relevant term. Note, however, note that the holon channels do not contribute to the desired term, which also appears at order  $J_H^2$ .

$$\begin{aligned} & \text{Hz3}[[2, 3, 1]] // \text{FullSimplify} \\ & \frac{1}{27 (2 J + U) (3 J^2 - 4 J U + U^2)^2} 4 i J^2 \\ & \quad \left( 2 J (3 t^2 (8 t_a + 5 t_s) - t_4 (-24 t_1 t_a + 8 t_3 t_a + 21 t_4 t_a + 10 t_1 t_s - 10 t_3 t_s + 9 t_4 t_s)) + \right. \\ & \quad \left. (3 t^2 (3 t_a + 5 t_s) - t_4 (26 t_1 t_a - 12 t_3 t_a + 6 t_4 t_a + 10 t_1 t_s - 10 t_3 t_s + 9 t_4 t_s)) U \right) \\ & \text{Hz3}[[2, 3, 1]] /. \{t_4 \rightarrow 0\} // \text{FullSimplify} \\ & \frac{4 i J^2 t^2 (16 J t_a + 10 J t_s + 3 t_a U + 5 t_s U)}{9 (2 J + U) (3 J^2 - 4 J U + U^2)^2} \end{aligned}$$

```

MatrixForm /@ Simplify[J^2 SeriesCoefficient[Hz3[[2, 3, 1]], {J, 0, 2}]] //
FullSimplify // Factor

$$\frac{4 i}{27} J^2 \left( 3 t^2 (3 t a + 5 t s) - t^4 (26 t_1 t a - 12 t_3 t a + 6 t_4 t a + 10 t_1 t s - 10 t_3 t s + 9 t_4 t s) \right) \frac{1}{U^4}$$

MatrixForm /@ Simplify[J^2 SeriesCoefficient[Hz3[[2, 3, 1]] /. {t4 -> 0}, {J, 0, 2}]] //
FullSimplify // Factor

$$\frac{4 i}{9} J^2 t^2 (3 t a + 5 t s) \frac{1}{U^4}$$

SessionTime[] - start
214.1218436

```

## 4-hop processes

Paths visiting three sites in four hops. First are  $c$  and  $c'$

$$H_{zc} = T^y \sigma T^x M^2 T^x M T^y \sigma \quad (\text{order } 2321)$$

```

Mzc = TJy.sigma6.TJx.MM2.TJx.MM.TJy;
Hzct = Sum[TensorProduct[TensorTranspose[Mzc, {1, 3, 4, 5, 2}][[aa, a]],
  TensorTranspose[sigma, {3, 1, 2}][[a, aa]]], {a, 1, 2}, {aa, 1, 2}];
Hzc = TensorTranspose[TensorMultiply[-i ee, Hzct, {{2, 1}, {3, 3}}], {2, 3, 1}];

```

$$H_{zcp} = T^x \sigma T^y M^2 T^y M T^x \sigma \quad (\text{order } 2123)$$

```

Mzcp = TJx.sigma6.TJy.MM2.TJy.MM.TJx;
Hzcpt = Sum[TensorProduct[TensorTranspose[Mzcp, {1, 3, 4, 5, 2}][[aa, a]],
  TensorTranspose[sigma, {3, 1, 2}][[a, aa]]], {a, 1, 2}, {aa, 1, 2}];
Hhcp = TensorTranspose[TensorMultiply[-i ee, Hzcpt, {{2, 1}, {3, 3}}], {2, 1, 3}];

```

And now  $(d)$  and  $(d')$

$$H_{zd} = T^x \sigma T^x M T^y M^2 T^y \sigma \quad (\text{order } 3212)$$

```

Mzd = TJx.sigma6.TJx.MM.TJy.MM2.TJy;
Hzdt = Sum[TensorProduct[TensorTranspose[Mzd, {1, 3, 4, 5, 2}][[aa, a]],
  TensorTranspose[sigma, {3, 1, 2}][[a, aa]]], {a, 1, 2}, {aa, 1, 2}];
Hzd = TensorTranspose[TensorMultiply[-i ee, Hzdt, {{2, 2}, {3, 4}}], {2, 3, 1}];
Hzdp = T^y \sigma T^y M T^x M^2 T^x \sigma \quad (\text{order } 1232)

```

```

Mzdp = TJy.sigma6.TJy.MM.TJx.MM2.TJx;
Hzdpt = Sum[TensorProduct[TensorTranspose[Mzdp, {1, 3, 4, 5, 2}][[aa, a]],
  TensorTranspose[sigma, {3, 1, 2}][[a, aa]], {a, 1, 2}, {aa, 1, 2}];
Hzdp = TensorTranspose[TensorMultiply[-i ee, Hzdpt, {{2, 2}, {3, 4}}], {2, 1, 3}];

```

```
Hz4 = Hzc - Hzcp + Hzd - Hzdp;
```

The term we wanted:

```
Hz4[[2, 3, 1]] // Simplify // Factor
```

$$-\left(\left(32 i J^2 (2 t_1 + t_3) t_4 (11 t_1 t_2 - 3 t_2^2 + t_2 t_3 + 4 t_1 t_4 + 2 t_3 t_4 + 3 t_4^2) (2 J - U)\right) / \left(81 (J - U)^3 (3 J - U)^3\right)\right)$$

```
SessionTime[] - start
```

```
239.5723919
```

It turns out that nothing appears until order  $J^2/U^5$  (This part of the calculation can take a few minutes due to the Simplify command)

```
Map[MatrixForm, 81 U^3 Hzc /. {J -> 0} // Simplify]
Map[MatrixForm, 81 U^4 SeriesCoefficient[Hz4, {J, 0, 1}] // Simplify]
```

$$\left\{\begin{pmatrix} 0 & 0 & 0 \\ 0 & 0 & 0 \\ 0 & 0 & 0 \end{pmatrix}, \begin{pmatrix} 0 & 0 & 0 \\ 0 & 0 & 0 \\ 0 & 0 & 0 \end{pmatrix}, \begin{pmatrix} 0 & 0 & 0 \\ 0 & 0 & 0 \\ 0 & 0 & 0 \end{pmatrix}\right\}$$

$$\left\{\begin{pmatrix} 0 & 0 & 0 \\ 0 & 0 & 0 \\ 0 & 0 & 0 \end{pmatrix}, \begin{pmatrix} 0 & 0 & 0 \\ 0 & 0 & 0 \\ 0 & 0 & 0 \end{pmatrix}, \begin{pmatrix} 0 & 0 & 0 \\ 0 & 0 & 0 \\ 0 & 0 & 0 \end{pmatrix}\right\}$$

```
SessionTime[] - start
```

```
422.2543262
```

The term we wanted appeared at order  $J^2/U^5$  but required  $t_4$  hopping, which breaks the ideal crystal symmetry. It turns out that there are other terms (that don't project to zero flux in the Kitaev model) that appear at this order  $J^2/U^5$  without the need for  $t_4$  (they do require  $t_2$ , however).

```
Map[MatrixForm, 81 U^5 SeriesCoefficient[Hz4 /. {t4 -> 0}, {J, 0, 2}] // Simplify]
```

$$\left\{\begin{array}{cc} 0 & 16 i t_2 (2 t_1 + t_3) (5 t_1^2 + 3 t_2^2 - 2 t_1 t_3 - 3 t_2 t_3) \\ 16 i t_2 (2 t_1 + t_3) (-3 t_1^2 + 3 t_2^2 + 2 t_1 t_3 + t_3^2) & 16 i t_2 (2 t_1 + t_3) (5 t_1^2 + 3 t_2^2 - 2 t_1 t_3 - 3 t_2 t_3) \\ 64 i t_2^2 (2 t_1 + t_3)^2 & 64 i (t_1^2 + t_2^2 - t_1 t_3) (2 t_1^2 - t_1 t_3 - t_3^2) \end{array}\right\}$$

```
SessionTime[] - start
```

```
571.9593467
```

Now I take care of some other types of 3-site, 4-hop processes that were not in Ko et al.

$Hze = T^y M T^x M T^x M T^y \sigma$  (order 2321)

```
Mze = TJy.MM.TJx.MM.TJx.MM.TJy;
Hzet = Sum[TensorProduct[TensorTranspose[Mze, {1, 3, 4, 5, 2}][[aa, a]],
  TensorTranspose[sigma, {3, 1, 2}][[a, aa]]], {a, 1, 2}, {aa, 1, 2}];
Hze = TensorTranspose[TensorMultiply[-i ee, Hzet, {{2, 1}, {3, 3}}], {2, 3, 1}];
```

Note that both  $(a_i)$  processes are their own time-reversal conjugates

$Hzf = T^x M T^y M T^y M T^x \sigma$  (order 2123)

```
Mzf = TJx.MM.TJy.MM.TJy.MM.TJx;
Hzft = Sum[TensorProduct[TensorTranspose[Mzf, {1, 3, 4, 5, 2}][[aa, a]],
  TensorTranspose[sigma, {3, 1, 2}][[a, aa]]], {a, 1, 2}, {aa, 1, 2}];
Hzf = TensorTranspose[TensorMultiply[-i ee, Hzft, {{2, 1}, {3, 3}}], {2, 1, 3}];
```

SessionTime[] - start

625.6284956

Up to now this notebook has taken 4.5 mins

This last evaluation takes ~15mins, but is an important result: The three spin terms in the (e) (f) channels vanish

```
Map[MatrixForm, Hze // Simplify]
```

```
Map[MatrixForm, Hzf // Simplify]
```

$$\left\{ \begin{pmatrix} 0 & 0 & 0 \\ 0 & 0 & 0 \\ 0 & 0 & 0 \end{pmatrix}, \begin{pmatrix} 0 & 0 & 0 \\ 0 & 0 & 0 \\ 0 & 0 & 0 \end{pmatrix}, \begin{pmatrix} 0 & 0 & 0 \\ 0 & 0 & 0 \\ 0 & 0 & 0 \end{pmatrix} \right\}$$

$$\left\{ \begin{pmatrix} 0 & 0 & 0 \\ 0 & 0 & 0 \\ 0 & 0 & 0 \end{pmatrix}, \begin{pmatrix} 0 & 0 & 0 \\ 0 & 0 & 0 \\ 0 & 0 & 0 \end{pmatrix}, \begin{pmatrix} 0 & 0 & 0 \\ 0 & 0 & 0 \\ 0 & 0 & 0 \end{pmatrix} \right\}$$

SessionTime[] - start

1490.0482309

Finally, I check what this second-neighbor hopping gives for (NNN) exchange constants.

We focus on a z-bond

```
H2 = 2 Sum[TensorProduct[TensorTranspose[sigma, {3, 1, 2}][[aa, a]], TensorTranspose[
  ConjugateTranspose[TJz2].MM.TJz2, {1, 3, 2}][[a, aa]]], {a, 1, 2}, {aa, 1, 2}];
```

```
Jterm2 = (H2[[1, 1]] + H2[[2, 2]]) / 2 // FullSimplify
```

$$-\frac{4 \, t a^2 \left( J^2 + J \, U - U^2 \right)}{9 \left( J - U \right) \left( 3 J - U \right) \left( 2 J + U \right)}$$

```
Kterm2 = Hz2[[3, 3]] - Jterm2 // FullSimplify
```

$$\frac{\left(4 \left(4 J^2 \left(t_a^2 + 3 t_a t_s + 3 t_s^2\right) + 3 J \left(t_a^2 + 2 t_a t_s + 2 t_s^2\right) U - 2 t_a^2 U^2\right)\right)}{\left(9 (J-U) (3 J-U) (2 J+U)\right)}$$

```
Γterm2 = Hz2[[1, 2]] // FullSimplify
```

```
0
```

```
Γpterm2 = Hz2[[1, 3]] // FullSimplify
```

```
0
```

Indeed we find Heisenberg exchange at  $J_H/J_K \sim (t_a/t_s)^2$
